# Supplementary material for: Emergence of colloidal patterns in AC electrical fields
Source: arXiv:2105.03590 source file (2021-05-08)
Supplement: Supplementary file 1 [file Katzmeier_SI.pdf]

# Emergence of colloidal patterns in AC electrical fields

## Supplementary Information

### 1 Materials & Methods

#### 1.1 Preparation of colloidal suspensions

In initial experiments, we found that the formation of patterns predominantly occurs at low salt concentrations (250  $\mu\text{M}$  NaCl). We therefore usually included several washing steps in the preparation of our colloidal sample. Distilled and deionized water (ddH<sub>2</sub>O) with a resistivity  $\rho$  of 18.2 M $\Omega$ /cm was obtained from a water purification system (Sartorius arium® pro).

##### 1.1.1 Silica micro spheres

Monodisperse silica particles with a diameter of 1.3  $\mu\text{m}$  in 5 % (w/v) aqueous suspension were purchased from the microParticles GmbH (LOT:SiO<sub>2</sub>-F-L1272). Before usage, we vortexed the stock solution and mixed 100  $\mu\text{L}$  of the stock solution with 900  $\mu\text{L}$  ddH<sub>2</sub>O in an Eppendorf tube. The sample was centrifuged in a table centrifuge for 30 s until the colloids sedimented completely. The excess washing liquid (900  $\mu\text{L}$ ) was then carefully removed again. The washing steps were repeated 5 times. The washed stock solution was then used as a starting solution for all further experiments with silica particles.

For the experiment shown in figure 1(b) of the main text we created a solution with a particle density of 0.0375 % (w/v) and a NaCl concentration of 250  $\mu\text{M}$ . A particle density of 0.0375 % (w/v) nominally corresponds to 176 210 particles per  $\text{mm}^3$ , where we used a density of 1.85 g/cm<sup>3</sup> [1] for silica. In order to generate more distinct macroscopic patterns, for the experiment shown in figure 1(c) we created a suspension with a higher particle density of 0.1 % (w/v) in a 250  $\mu\text{M}$  NaCl solution.

##### 1.1.2 Polyallylamine-ATP coacervates

Polyallylamine with an average molecular weight of 17 kDa was obtained as an aqueous solution with a concentration of 20 % (w/w) (Sigma Aldrich 479136-1G, Lot # MKCL0467). We diluted the polyallylamine solution to a monomer concentration of 20 mM and adjusted the pH to 7. Adenosine 5'-triphosphate (ATP) dipotassium salt (Sigma Aldrich A8937-1G, Lot # SLBP7423V) was used to create a 100 mM stock solution in ddH<sub>2</sub>O, which we aliquoted and froze at  $-20^\circ\text{C}$ . The conditions for the formation of stable polyallylamine-ATP coacervate droplets were derived from [2]. To create the coacervates we pipetted 20  $\mu\text{L}$  of the ATP stock into 1000  $\mu\text{L}$  of

the polyallylamine stock solution which was kept at 4 °C and vortexed the solution briefly. We then centrifuged the sample at 10000 rcf and 4 °C for 1 min. We then removed the supernatant and resuspended the coacervates in 1 mL ddH<sub>2</sub>O. After a second washing step the coacervates were resuspended in 500 µL of a 250 µM NaCl solution.

### **1.1.3 Molten lauric acid droplets**

0.5 mg lauric acid (Sigma Aldrich, # W261408-SAMPLE-K) was added to 10 mL of a 250 µM NaCl solution in a 15 mL Falcon tube. The Falcon tube was placed in a water bath placed on a heat plate, which had been set to 150 °C for 30 min. When the lauric acid was dissolved, we vortexed the Falcon tube for 1 min and diluted 100 µL of the resulting lauric acid emulsion in 900 µL of a pre-heated 250 µM NaCl solution in an Eppendorf tube. The sample was vortexed again for 1 min and a 100 µL aliquot was diluted once more in 900 µL of a pre-heated NaCl solution. We then sonicated the sample for 1 min using an ultrasonic homogenizer (Bandelin Sonopuls mini20) equipped with an MS 2.5 sonotrode at maximum settings (20 W). The sonotrode was moved in circles around the liquid air interface near the wall of the tube (this was done as we found that the colloids tended to accumulate at that part of the tube during sonication). After preparation, the sample was stored in the heat bath.

### **1.1.4 Fluorocarbon oil droplets**

2 µL fluorocarbon oil (Sigma Aldrich, # F9755) containing 2% of a surfactant (FluoSurf from Emulseo, Bordeaux) was added to 998 µL of a 250 µM NaCl solution. We sonicated the sample for 1 min at maximum power (20 W). As for the lauric acid droplets, the sonotrode was moved in circles around the liquid air interface near the wall of the tube.

### **1.1.5 E.coli bacteria**

Bacteria (E.coli DH5α) were grown for 16 h at 36 °C in 5 mL of LB medium (Carl Roth, # X968.1) in a shaking incubator. The bacteria were diluted 1 to 100 in two tubes each containing 5 mL of fresh LB medium and grown until an OD<sub>600</sub> of 2.1 was reached. The tubes containing the bacteria were put on ice for 15 min to cool them down to 4 °C, followed by centrifugation at 3000 rcf and 4 °C for 15 min. The supernatant was removed and the bacterial pellets were resuspended each in 5 mL of 4 °C cold ddH<sub>2</sub>O. After two further washing steps the bacteria were eluted in 1 mL of a 250 µM NaCl solution and pooled.

### 1.1.6 Coffee

Coffee was brewed in the office with a filter coffee machine using 2 spoons of ground coffee (Dallmayr Prodomo, 100% ARABICA) and 2 coffee filters (Rewe, Ja!). The coffee was filled into a 0.2 L cup, which was placed on an office desk and covered with a piece of carton. After letting the coffee particles sediment for 24 h, we recovered the cold coffee suspension from the office desk. To this end, we removed two times 5 mL of the coffee suspension from the surface of the cup and put them in two 15 mL Falcon tubes. We then followed the same washing protocol used for the bacteria. We sonicated the final coffee samples for 1 min at maximum settings (20 W) to remove any remaining larger coffee particles.

## 1.2 Microscopy experiments

AC signals of up to 20 V peak to peak were generated with a function generator RIGOL DG812 and were amplified with a home-built two channel, bipolar amplifier to voltages in the range  $[-290 \text{ V} : 290 \text{ V}]$ . Each amplifier channel employs a pair of high voltage operational amplifiers (Apex PA443) connected in a bridge amplifier configuration with a gain adjusted to 36 (31.1 dB). Due to the employed operational amplifier and circuit configuration, the maximum slew rate is limited to  $64 \text{ V}/\mu\text{s}$ . Detailed schematics and circuit board layouts can be provided by the authors upon request.

We conducted our experiments in self-made glass chambers or in commercial plastic chambers (Ibidi,  $\mu$ -Slide VI 0.4), depending on the physical nature of our colloids. The self-made glass chambers are an adaption of the design used by Kopperger and List. [3] Details can be provided by the authors upon request. For imaging, we used an inverted microscope (Olympus IX71) equipped with a CCD camera (Andor Luca, DL-604M). Self-made glass chambers enabled us to apply larger electric fields due to their shorter channel length, which we found to be necessary to trigger the formation of patterns for coffee particles, E.coli and fluorocarbon oil. On the other hand, we avoided to measure lauric acid and silica micro spheres in glass chambers as they tended to stick to the glass surface. The specific experimental conditions are listed in table 1. In all experiments, we used sample volumes of  $100 \mu\text{L}$  of the colloidal suspensions described above. For the experiment with lauric acid we used a temperature controlled microscopy stage (Tokai Hit OLYMPUS THERMO PLATE, #MATS-UAXKP-D) which was heated to  $50^\circ\text{C}$ . The nominal exposure time was set to 50 ms in our experiments. The actual time be-

tween frames was saved in the metadata file and was  $\approx 100$  ms. The scale bar of the images in figure S1 and the time stamp of the supplementary videos was inserted with ImageJ.

**Table 1: Experimental settings for imaging the different colloids**

| Colloid           | Channel | Channel length (mm) | Voltage amplitude (V) | Electric field amplitude (mV/ $\mu$ m) | Frequency (Hz) | Objective |
|-------------------|---------|---------------------|-----------------------|----------------------------------------|----------------|-----------|
| Silica (Fig. 1 B) | Ibidi   | 17                  | 288                   | 17                                     | 500            | 40x       |
| Silica (Fig. 1 C) | Ibidi   | 17                  | 288                   | 17                                     | 500            | 20x       |
| Coacervates       | Ibidi   | 17                  | 288                   | 17                                     | 500            | 10x       |
| Lauric acid       | Ibidi   | 17                  | 288                   | 17                                     | 500            | 10x       |
| Fluocarbon oil    | Glass   | 5                   | 180                   | 36                                     | 500            | 20x       |
| Coffee            | Glass   | 5                   | 288                   | 58                                     | 500            | 20x       |
| E. coli           | Glass   | 5                   | 288                   | 58                                     | 250            | 20x       |

### 1.2.1 Bacteria

In contrast to the experiments with the other colloids, for E.coli bacteria we found only vertical chain formation at an electric field frequency of 500 Hz. By contrast, the usual horizontal band structures were found at a lower frequency of 250 Hz. We attribute this finding to the presumably more complex electric properties of the bacteria. Two images of a bacterial suspension at the two frequencies are shown in Figure S1.

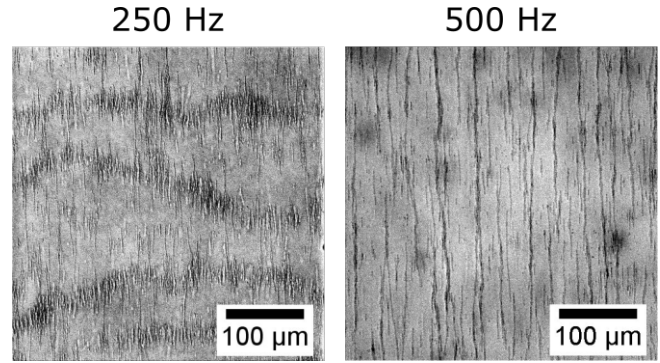

Figure 1: Both images are taken 100 s after the electric field was turned on. The other conditions are the same as listed in table 1. The electric field oscillates as usual along the vertical axis.

### 1.2.2 Imaging of the hydrodynamic flow (Fig. 3B)

In experiments with polydisperse particle suspensions we found that the hydrodynamic flow can be explicitly observed around larger particles based on the trajectory of the smaller particles surrounding them. To image the hydrodynamic flow we conducted an experiment with coacervates in a glass chamber where we applied an electric field amplitude of 36 mV/ $\mu$ m and a frequency of 500 Hz. Our coacervates were best suited for this experiment, as the corresponding samples usually contained a small number of larger particles. We recorded a video focused on a large coacervate with a 100x magnification. We corrected for the drift of the large coacer-

vate with an ImageJ plugin (Template Matching and Slice Alignment from Qingzong Tseng [4]). To create the image in Figure 3(b) we cut out a  $50 \times 50 \mu\text{m}^2$  region of the drift corrected video and computed the absolute difference of subsequent images of the stack, which lets moving particles appear as bright spots with high contrast. From this we computed the average of 30 successive video frames that had sufficient image quality. Particle trajectories appear as bright stripes in the averaged image.

## 2 Parameter screening

We explored the dependence of the emergence of patterns on AC field frequency and salt concentration to gain deeper insight into the underlying mechanism.

### 2.1 Experiment

For the experiment we prepared a washed silica particle stock solution as described in section 1.1.1, from which we generated suspensions at 0.0375 % (w/v) with NaCl concentrations ranging from 0  $\mu\text{M}$  to 2500  $\mu\text{M}$ . As the solution conductivity is a critical parameter of our experiment we prepared our experiments with particular care to avoid any salt contamination. Hence, before usage we washed every tube with ddH<sub>2</sub>O, and we multiply pipetted ddH<sub>2</sub>O with every fresh pipette tip before pipetting a sample. We flushed the commercial microscopy channels with ddH<sub>2</sub>O before filling them with a sample. We found that any contact of a sample with unwashed surfaces resulted in an increase in conductivity. We applied a relatively weak electric field with amplitude 10.6 mV/ $\mu\text{m}$  and applied frequencies ranging from 250 Hz to 25 kHz. Between successive runs at a fixed frequency, an electric field of 1.06 mV/ $\mu\text{m}$  at 1 Hz was applied for 2 min to mix the sample, followed by a pause of three minutes before the next run at a different frequency. We recorded microscopy videos with 2000 frames each and an exposure time of 50 ms/frame for every sample at a given frequency and salt concentration. The actual time interval between frames was around 100 ms and varied slightly from run to run. The actual time interval was saved in the microscopy metadata file and used later for the data analysis.

To confirm the absence of contaminants in a freshly prepared sample, we measured the conductivity of our samples at the lowest frequency (250 Hz) and compared it to the theoretically expected conductivity at a given salt concentration. To this end, we put a reference resistor  $R_{\text{ref}}$  in series with our sample and monitored the voltage across the resistor  $A(t)$  and the voltage supply  $B(t)$  with a digital oscilloscope (picoscope 2206B). We recorded  $\langle |A(t)| \rangle_T$ ,  $\langle |B(t)| \rangle_T$  and  $\langle A(t) \cdot B(t) \rangle_T$ . From this measurement, the conductivity of the sample can be determined

as follows:

The fraction of the voltage across the reference resistor that is in phase with the applied voltage is given by  $\frac{\langle A(t) \cdot B(t) \rangle_T}{\langle |B(t)| \rangle_T}$  and the corresponding in-phase current is  $\frac{\langle A(t) \cdot B(t) \rangle_T}{R_{\text{ref}} \langle |B(t)| \rangle_T}$ . From the latter we can compute the resistance of the sample via  $\frac{1}{R_{\text{sample}}} = \frac{\langle A(t) \cdot B(t) \rangle_T}{R_{\text{ref}} (\langle |B(t)| \rangle_T)^2}$  where we assumed that the resistance of the sample is much larger than that of the reference resistor. The electrolytic conductivity can be computed from  $R_{\text{sample}}$  and the channel geometry via  $\frac{1}{\rho} = \frac{1}{R_{\text{sample}}} \frac{L}{W \cdot H}$  where 17 mm, 3.8 mm and 0.4 mm. The measured data and the corresponding values for the in-phase current and electrolytic conductivity are listed in Table 2.

| [NaCl] ( $\mu\text{M}$ ) | $\langle  A(t)  \rangle_T$ (mV) | $\langle  B(t)  \rangle_T$ (V) | $\langle  A(t)B(t)  \rangle_T$ (V · V) | $R_{\text{ref}}$ $\Omega$ | In phase current ( $\mu\text{A}$ ) | $\frac{1}{\rho}$ $\mu\text{S}/\text{cm}$ |
|--------------------------|---------------------------------|--------------------------------|----------------------------------------|---------------------------|------------------------------------|------------------------------------------|
| Air                      | 6.85                            | 125.9                          | 0.007                                  | 11000                     | 0.0051                             | 0.0045                                   |
| 0                        | 8.467                           | 125.9                          | 0.98                                   | 11000                     | 0.71                               | 0.63                                     |
| 5                        | 20.01                           | 126                            | 2.47                                   | 11000                     | 1.78                               | 1.58                                     |
| 10                       | 26.68                           | 125.9                          | 3.331                                  | 11000                     | 2.41                               | 2.14                                     |
| 25                       | 50.63                           | 125.8                          | 6.362                                  | 11000                     | 4.60                               | 4.09                                     |
| 50                       | 96.26                           | 125.9                          | 12.11                                  | 11000                     | 8.74                               | 7.77                                     |
| 100                      | 171.8                           | 126                            | 21.64                                  | 11000                     | 15.61                              | 13.86                                    |
| 250                      | 396                             | 126                            | 50.08                                  | 11000                     | 36.13                              | 32.07                                    |
| 500                      | 841                             | 125.9                          | 105.9                                  | 11000                     | 76.47                              | 67.93                                    |
| 1000                     | 171.6                           | 125.9                          | 21.72                                  | 1100                      | 156.83                             | 139.32                                   |
| 2500                     | 357                             | 125.9                          | 45.89                                  | 1100                      | 331.36                             | 294.36                                   |

Table 2: Measurements of the electrolytic conductivity  $\frac{1}{\rho}$  of the microscopy samples used for the screening experiment.

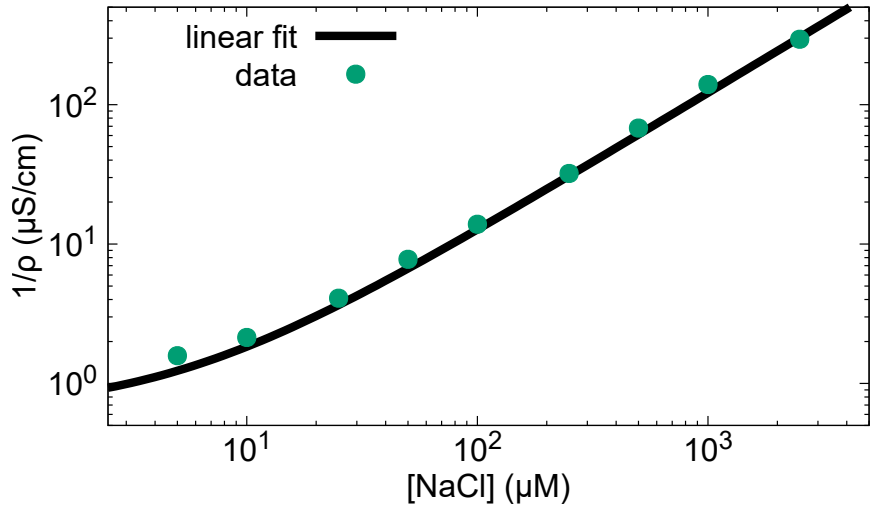

Figure 2: Plot of the electrolytic conductivity  $\frac{1}{\rho}$  from Table 2 fitted to a linear function.

We fitted a line to the measured conductivity values to obtain the limiting conductivity  $\Lambda$  from the extrapolated value of  $\frac{1}{\rho}$  at 0  $\mu\text{M}$  (Figure 2). We found  $\Lambda = 0.121$  (S/cm)/M which is in good agreement with the theoretical value for the limiting conductivity of 0.125 (S/cm)/M computed from the Nernst-Einstein equation (using  $D_{\text{Na}^+} = 1.3 \times 10^{-9} \text{m}^2/\text{s}$  and  $D_{\text{Cl}^-} = 2 \times 10^{-9} \text{m}^2/\text{s}$ ).

### 2.1.1 Data analysis

We defined the ‘pattern visibility’  $p$  of a pattern in an image as a measure for large scale structure occurring along the direction of the electric field, i.e., in  $z$ -direction. To obtain  $p$  we first apply a Gaussian filter with a standard deviation of 15 pixels (corresponding to  $6\text{ }\mu\text{m}$  at our magnification) to an image. This eliminates the information of individual particles. Images of a pattern will have large scale density fluctuations in  $z$ -direction while images with no pattern will appear mostly homogeneous. The density fluctuations can be quantified by computing the absolute value of the derivative of the image in  $z$ -direction. We then sum over the whole image. In practice, this amounts to the calculation of a discretized version of

$$p = \int_A \left| \frac{\partial}{\partial z} (G * I)(x, z) \right| dx dz \quad (1)$$

where  $g$  is a Gaussian function and  $I$  is the intensity of the image ( $*$  indicates convolution). We computed  $p$  for every frame of the videos of our screening experiment. We then computed the speed of the patterning process  $\tau_p^{-1}$  by fitting lines to the initial stage of the  $p$  vs time data. Examples of the  $p$  vs time data including the linear fit are shown in figure 3.

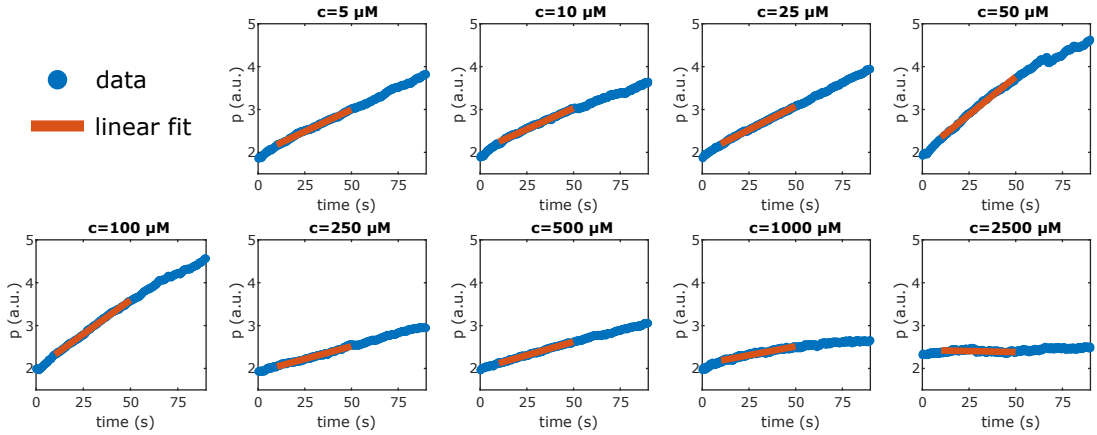

Figure 3: Example plots of the  $p$  vs time data for 250 Hz measurements. The linear fit to obtain the initial speed  $\tau_p^{-1}$  of the patterning process is also included.

We analyzed our microscopy videos with ImageJ scripts. To compute the derivative of an image we used the FeatureJ plugin.

## 3 Theory and Simulation

The SDE governing the particle dynamics in explicit form is given by

$$a d\mathbf{q}_i = u^* \sum_{j \neq i} \left[ \xi^2 \left( \frac{\gamma}{2} \mathbf{g}(\mathbf{r}_{ij}) + (|K_d|^2 - \gamma) \mathbf{h}(\mathbf{r}_{ij}) \right) + \nu \mathbf{k}(\mathbf{r}_{ij}) \right] dt + \sqrt{2D_p} dW_i. \quad (2)$$

where the particle distance  $\mathbf{r}_{ij}$  are defined by  $\mathbf{r}_{ij} = \mathbf{q}_i - \mathbf{q}_j$  and  $dW_i$  is the stochastic increment of a Wiener process. The positions of the particles centers  $\mathbf{q}_i$  are given in dimensionless variables (multiple particle radii). For the purpose of our simulation we re-scaled time by  $\frac{a^2}{D_p}$  and introduced the new dimensionless numbers

$$\alpha = \frac{\gamma}{2} \frac{a}{D_p} \xi^2 u^*, \quad (3)$$

$$\beta = (|K_d^2| - \gamma) \frac{a}{D_p} \xi^2 u^* \quad (4)$$

and

$$\tilde{\nu} = \nu \frac{a}{D_p} u^*. \quad (5)$$

With this the SDE is given by

$$d\mathbf{q}_i = \sum_{j \neq i} \left[ \alpha \mathbf{g}(\mathbf{r}_{ij}) + \beta \mathbf{h}(\mathbf{r}_{ij}) + \tilde{\nu} \mathbf{k}(\mathbf{r}_{ij}) \right] dt + \sqrt{2} dW_i. \quad (6)$$

The repulsion force  $\mathbf{k}(\mathbf{r}_{ij})$  is included for particles in contact with each other. Particles are in contact when they are closer than two times the particle radius  $a$ . In dimensionless variables this condition is given by  $|\mathbf{r}_{ij}| = |\mathbf{q}_i - \mathbf{q}_j| < 2$ . The dipole-dipole-force and the hydrodynamic-interactions are only defined outside the particles. We therefore assume that these interactions do not increase any further for intersecting particles. We halt  $\mathbf{h}$  and  $\mathbf{g}$  at their value at the particle surface and thereby obtain continuous vector fields. The explicit expressions for the particle interactions used in the simulation are given by

$$\mathbf{g}(\mathbf{r}) = \begin{cases} \frac{(1-3\cos^2(\theta))}{r^2} \hat{\mathbf{e}}_r & \text{for } r > 2 \\ \frac{(1-3\cos^2(\theta))}{2^2} \hat{\mathbf{e}}_r & \text{for } r \leq 2 \end{cases} \quad (7)$$

$$\mathbf{h}(\mathbf{r}) = \begin{cases} \frac{1-3\cos^2(\theta)}{r^4} \hat{\mathbf{e}}_r - \frac{2\cos(\theta)\sin(\theta)}{r^4} \hat{\mathbf{e}}_\theta & \text{for } r > 2 \\ \frac{1-3\cos^2(\theta)}{2^4} \hat{\mathbf{e}}_r - \frac{2\cos(\theta)\sin(\theta)}{2^4} \hat{\mathbf{e}}_\theta & \text{for } r \leq 2 \end{cases} \quad (8)$$

and

$$\mathbf{k}(\mathbf{r}) = \begin{cases} 0 & \text{for } r > 2 \\ \frac{1}{\sqrt{2}} (2-r)^{\frac{3}{2}} \hat{\mathbf{e}}_r & \text{for } r \leq 2 \end{cases} \quad (9)$$

### 3.1 Simulation

We implemented the Euler-Maruyama solution scheme to solve the overdamped many particle Langevin equation numerically. We explicitly compute

$$\delta \mathbf{q}_i^t = \sum_{j \neq i} \left[ \alpha \mathbf{g}(\mathbf{r}_{ij}^t) + \beta \mathbf{h}(\mathbf{r}_{ij}^t) + \tilde{\nu} \mathbf{k}(\mathbf{r}_{ij}^t) \right] \delta t + \sqrt{2\delta t} \mathbf{X}_i \quad (10)$$

for every time step  $\delta t$  where  $\mathbf{X}_i$  is a two-component vector of normally distributed random numbers with standard deviation 1 and  $\mathbf{r}_{ij}^t$  is defined by  $\mathbf{r}_{ij}^t = \mathbf{q}_i^t - \mathbf{q}_j^t$ . This in turn gives the updated particle positions via

$$\mathbf{q}_i^{t+\delta t} = \mathbf{q}_i^t + \delta \mathbf{q}_i^t \quad (11)$$

### 3.2 Implementation

The particles are placed on a square grid with a dimensionless distance of  $d = 5.6$ . We choose the grid distance in such a way that the particle density is matched with our screening simulation. This is explained in more detail in section 3.4.

We begin our simulations by letting the particles diffuse freely with only the repulsion force acting between particles. We increased the standard deviation of the random number by a factor of 10 for a more rapid randomization and let the particles diffuse for 2000 integration steps with  $\delta t = 1 \times 10^{-3}$ . We explicitly compute

$$\delta \mathbf{q}_i^t = \sum_{j \neq i} \left[ \tilde{\nu} \mathbf{k}(\mathbf{r}_{ij}^t) \right] \delta t + 10 \sqrt{2\delta t} \mathbf{X}_i. \quad (12)$$

This gives a mean square displacement for a particle from the initial position of approximately 400. The parameters of this initial stage are chosen such that  $\sqrt{400}$  is larger compared to the initial particle distance and therefore yields a sufficient randomization of the particle positions.

After the randomization, the particle positions are updated according to equation (10) and (11). We implemented periodic boundary conditions by surrounding the 2D simulation box with eight copies of itself. The forces acting on one particle are computed by considering all other particles including the eight copies. Particles moving out of the simulation box on one side re-enter the box from the opposite side.

### 3.3 Numerical stability

We observed that for badly chosen simulation parameters, particles tend to diffuse into each other and are then subjected to a large repulsion force which makes them jump over unphysically large distances. We therefore determined ad hoc criteria for the repulsion parameter  $\tilde{\nu}$  of the contact force and the time step  $\delta t$  to prevent this particle hopping artifact. To this end, we first consider the equilibrium position of two intersecting particles. The maximum attraction of the two vector fields  $\alpha \mathbf{h}$  and  $\beta \mathbf{g}$  is given at an angle  $\theta = 0$  and a distance  $r = 2$ . We thus find  $\max(-\alpha \mathbf{g}) = \frac{\alpha}{2}$  and  $\max(-\beta \mathbf{h}) = \frac{\beta}{8}$ . The equilibrium position of two intersecting particles at

maximum attraction is therefore given by

$$r_m = 2 - \left( \frac{\sqrt{2}}{\tilde{\nu}} \left( \frac{\beta}{8} + \frac{\alpha}{2} \right) \right)^{\frac{2}{3}} \quad (13)$$

For our large scale simulation we choose  $\alpha = 7$  and  $\beta = 35$ , and  $\tilde{\nu} = 400$ , which gives  $r_m = 1.91$ , corresponding to a 4.6 % deviation from the hard sphere distance.

Particle hopping occurs when a particle diffuses far enough into another particle's core such that the resulting repulsion force displaces the particle over a large distance away from the other particle. Lets say one particle has diffused far into an other particle such that their centers have now the distance  $|r| < 2$ . In the next integration step the particle will be displaced by the distance  $\tilde{\nu}k(r)\delta t$ . We want to avoid that the particle is catapulted out of the other particle. We therefore require that the particle does not leave the other particle in one single integration step. Such an integration step is at least  $|2 - r|$  long. We therefore require

$$|2 - r| > \tilde{\nu} \frac{1}{\sqrt{2}} (2 - r)^{\frac{3}{2}} \delta t, \quad (14)$$

which gives

$$\sqrt{2 - r} > \frac{\sqrt{2}}{\tilde{\nu}\delta t}. \quad (15)$$

We now require such a jump to be extremely unlikely. ( $\leq 10 \sigma$  or  $p \leq 1.5 \times 10^{-23}$ ):

$$10\sqrt{2\delta t} = |2 - r|, \quad (16)$$

which in combination with equation 15 results in a condition for the maximum time step of our simulation:

$$\delta t = \left( \frac{\sqrt{2}}{10\tilde{\nu}^2} \right)^{\frac{2}{5}} \quad (17)$$

For  $\tilde{\nu} = 400$ , this conditions yields  $\delta t = 4.7 \times 10^{-3}$ , and we therefore choose the slightly smaller value of  $\delta t = 1 \times 10^{-3}$ .

### 3.4 Matching the particle density between experiment and simulation

The particles in our simulation are initially placed on a square grid with a defined distance  $d$  between particles.  $d$  is related to the 2D particle density  $C_A$  via  $C_A = \frac{1}{d^2}$  or  $d = \sqrt{\frac{1}{C_A}}$ . We estimate  $C_A$  in our screening experiment by counting the particles in the first frame of a video. For every concentration of NaCl we randomly choose one experiment at a given frequency for counting, and count the particles in a  $(100 \mu\text{m})^2$  large part of an image. The results are shown

in Table 3.4. We find an average particle number of 763 which corresponds to a dimensionless particle density of 0.0322. We used  $100\text{ }\mu\text{m} \hat{=} 153.8$  for rescaling space with the particle radius of  $a = 0.65\text{ }\mu\text{m}$ . For the dimensionless particle distance we find  $d = 5.6$ .

From the previously computed particle density of 176 210 per  $\text{mm}^3$  and the channel height of 0.4 mm we would expect 705 particles in an area of  $(100\text{ }\mu\text{m})^2$  (this 10% deviation from the expected value presumably is the result of the particle washing procedure).

|                                           |     |     |      |     |       |      |     |       |       |      |
|-------------------------------------------|-----|-----|------|-----|-------|------|-----|-------|-------|------|
| Concentration ( $\mu\text{M}$ )           | 0   | 5   | 10   | 25  | 50    | 100  | 250 | 500   | 1000  | 2500 |
| Frequency (Hz)                            | 750 | 750 | 7500 | 250 | 17500 | 1000 | 250 | 12500 | 15000 | 2500 |
| Particles in $(100\text{ }\mu\text{m})^2$ | 755 | 767 | 690  | 820 | 779   | 803  | 750 | 681   | 826   | 759  |

Table 3: Counted number density of particles in our screening experiment

## References

- [1] Properties | microparticles gmbh. <https://microparticles.de/en/properties.html>, 23.07.2020.
- [2] Erica A. Frankel, Philip C. Bevilacqua, and Christine D. Keating. Polyamine/nucleotide coacervates provide strong compartmentalization of  $\text{Mg}^{2+}$ , nucleotides, and rna. *Langmuir : the ACS journal of surfaces and colloids*, 32(8):2041–2049, 2016.
- [3] Enzo Kopperger, Jonathan List, Sushi Madhira, Florian Rothfischer, Don C. Lamb, and Friedrich C. Simmel. A self-assembled nanoscale robotic arm controlled by electric fields. *Science*, 359(6373):296–301, 2018.
- [4] Qingzong Tseng, Irene Wang, Eve Duchemin-Pelletier, Ammar Azioune, Nicolas Carpi, Jie Gao, Odile Filhol, Matthieu Piel, Manuel Théry, and Martial Balland. A new micropatterning method of soft substrates reveals that different tumorigenic signals can promote or reduce cell contraction levels. *Lab on a chip*, 11(13):2231–2240, 2011.
